# Supplementary material for: Harnessing magnetic anisotropy for nonlinear magnetization precession and spin waves
Source: arXiv:2602.21796 ancillary file (2026-05-27)
Supplement: Supplementary file 1 [file supplemental.pdf]

# Harnessing magnetic anisotropy for nonlinear magnetization precession and spin waves: Supplementary Materials

P. I. Gerevenkov,* L. A. Shelukhin, Ia. A. Filatov, P. A. Dvortsova, and A. M. Kalashnikova

*Ioffe Institute, 194021 St. Petersburg, Russia*

(Dated: February 22, 2026)

## I. EXPERIMENTAL DETAILS

Time-resolved measurements were performed using an all-optical pump-probe method. All measurements were made at room temperature $T_0 = 295$ K. The out-of-plane magnetization dynamics was measured in the polar magneto-optical Kerr effect geometry, while an external field $H_{\mathrm{ext}}$ was applied in the sample plane.

For magnetization precession measurements $Yb^{3+}$:KGd$(WO_4)_2$ femtosecond regenerative amplifier PHAROS (Light Conversion) was used as a source of pump and probe pulses with duration $\tau = 190$ fs at a repetition rate 100 kHz. Pump pulses with wavelength 1030 nm (1.2 eV) and fluence 14 mJ·cm$^{-2}$ were focused at the 15° on the sample surface in the spot with diameter of 40 $\mu$m. Probe pulses had normal incidence in the area of 30 $\mu$m and wavelength 515 nm obtained from the same pulses with $\beta$-$BaB_2O_4$ crystal.

The measurement of propagating packets of surface spin waves was performed using the femtosecond oscillator laser TEMA (Avesta) with 190 fs pulses at a repetition rate 80 MHz. A wavelengths and fluence of pump pulse was 680 nm (1.8 eV) and 39 mJ·cm$^{-2}$, respectively. The probe pulse were 525 nm with at least 20 times less fluence. In this case, the femtosecond oscillator laser TEMA (Avesta) was used producing 150 fs pulses at a repetition rate 80 MHz. In order to excite spin waves at nonzero wavevector pump pulses were tightly focused (FWHM $\approx 0.9\mu$m). The propagating wave packets were spatially scanned along the direction perpendicular to the external field (Damon-Eshbach geometry).

## II. MICROMAGNETIC SIMULATION OF LASER-INDUCED SURFACE SPIN WAVE PACKET

The micromagnetic simulations presented in Fig. S.1 were performed using mumax3 [1] to model the generation and propagation of magnetostatic waves in a 20-nm-thick iron film following pulsed optical excitation. All simulations were conducted using material parameters, external magnetic field value and orientation, and laser excitation conditions that exactly matched those of the experiment described in the main text. The simulation domain was discretized using cubic cells with a side length of 20 nm in all spatial directions. While this cell size exceeds the exchange length of iron (approximately 2 nm), it remains significantly

* petr.gerevenkov@mail.ioffe.ru; http://www.ioffe.ru/ferrolab/

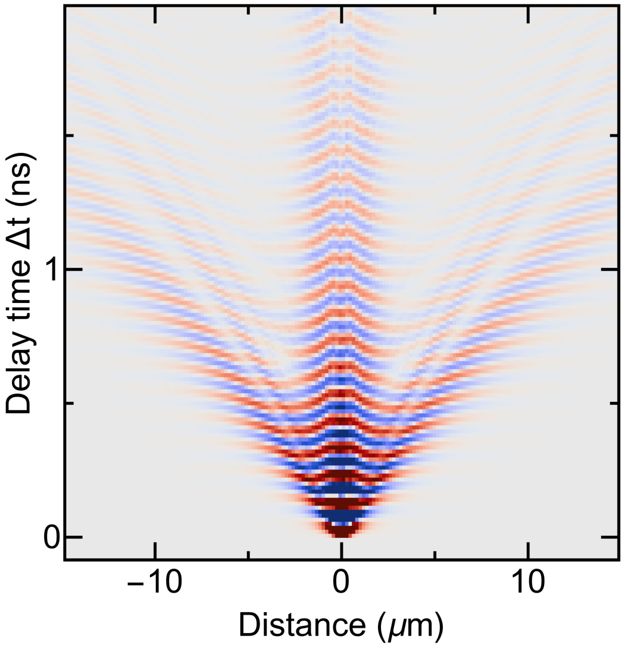


FIG. S.1. Map of pump-probe signal vs distance and delay time ($\Delta t$) between excitation and detection. The simulation parameters correspond to those used in the experiment shown in Fig. 3 b of the main text.

smaller than all characteristic wavelengths of the magnetostatic waves under investigation. Since the analysis focuses on magnetostatic, rather than exchange-dominated, spin waves, the use of a cell size larger than the exchange length does not affect the validity of the results. The excitation mechanism was implemented (see details in [2]) as an instantaneous modification of $M_S$ and $K_C$ with a Gaussian spatial profile, centered at the excitation region. Subsequently, both parameters relaxed back to their initial values following a power-law dependence with a characteristic time constant of 1.55 ns. To directly compare with the experimental geometry in the main text, the out-of-plane component of the magnetization was recorded as a function of time and position along the direction perpendicular to the applied magnetic field.

## III. SURFACE SPIN WAVES OUTSIDE THE EXCITATION REGION

To isolate the propagating spin wave signal from the signal within the excitation region, the detected magneto-optical response was multiplied by spatial weighting coefficients. The

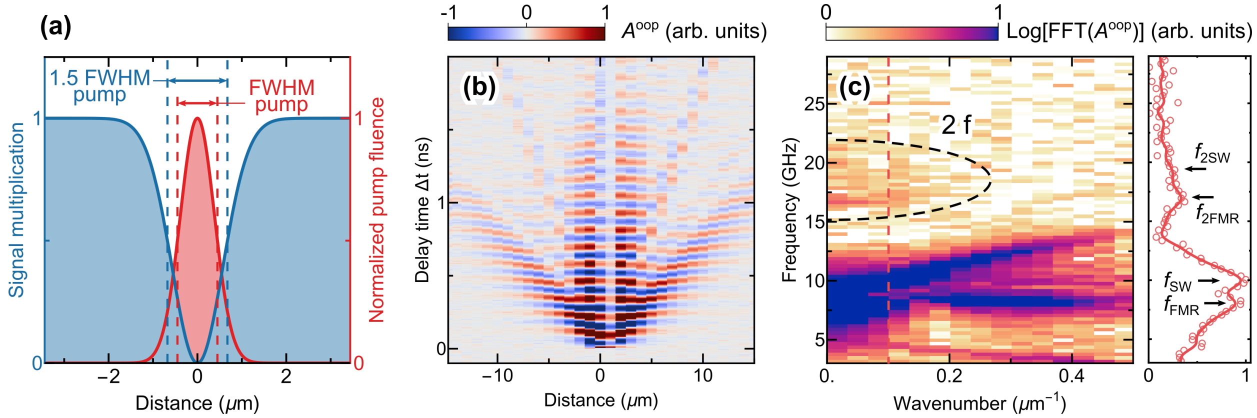


FIG. S.2. **Suppression of the excitation region signal for propagating wave analysis.** (a) Normalized spatial profiles of the pump energy density (red line) and the weighting coefficients $1 - G(x)$ (blue line) used to multiply the detected signal. The Gaussian weighting function $G(x)$ has a FWHM of 1.5 FWHM of the pump spot. (b) Magneto-optical response map after applying the weighting coefficients, analogous to Fig. 3 (c) of the main text. The signal from the excitation region is effectively suppressed, revealing propagating wave packets. (c) Dispersion relation of the data in panel (b). The right panel shows a cross-sections at $k = 0.1\,\mu\text{m}^{-1}$.

weighting coefficients were calculated as $1-G(x)$, where $G(x)$ is a Gaussian function centered at the excitation region with a full width at half maximum (FWHM) equal to 1.5 times the FWHM of the pump spot. Since the convolution of the pump and probe spot profiles results in an effective spatial resolution of $\sqrt{2}$ times the pump FWHM, this weighting procedure ensures that only the signal propagating beyond the excitation region is analyzed.

Figure S.2 a shows the normalized spatial profiles of the pump energy density and the resulting weighting coefficients. Figure S.2 b presents the magneto-optical response map, analogous to Fig. 3 (c) of the main text, after multiplication by the weighting coefficients. The dispersion relation obtained by applying a two-dimensional Fourier transform to the data in panel (b) is shown in Fig. S.2 c. The signal at the doubled frequency is clearly preserved. The right panel of Fig. S.2 c shows a cross-sections at $k = 0.1\,\mu\text{m}^{-1}$, revealing both the signal at the doubled ferromagnetic resonance frequency and the signal at the

doubled frequency of the surface spin wave.

[1] A. Vansteenkiste, J. Leliaert, M. Dvornik, M. Helsen, F. Garcia-Sanchez, and B. Van Waeyenberge, The design and verification of mumax3, AIP advances **4**, 10.1063/1.4899186 (2014).

[2] P. Gerevenkov, I. A. Filatov, A. Kalashnikova, and N. Khokhlov, Unidirectional propagation of spin waves excited by femtosecond laser pulses in a planar waveguide, Physical Review Applied **19**, 024062 (2023).
